# Supplementary material for: Towards Practical Few-shot Federated NLP
Source: arXiv:2212.00192 source file (2023-08-19)
Supplement: Supplementary file 1 [file sec-appendix-niid.tex]

\subsection{Definition of non-iid}\label{sec:appendix-niid}
\subsubsection{Non-IID. Label Distribution}
\begin{figure}[t]
	\centering
	 \includegraphics[width=0.45\textwidth]{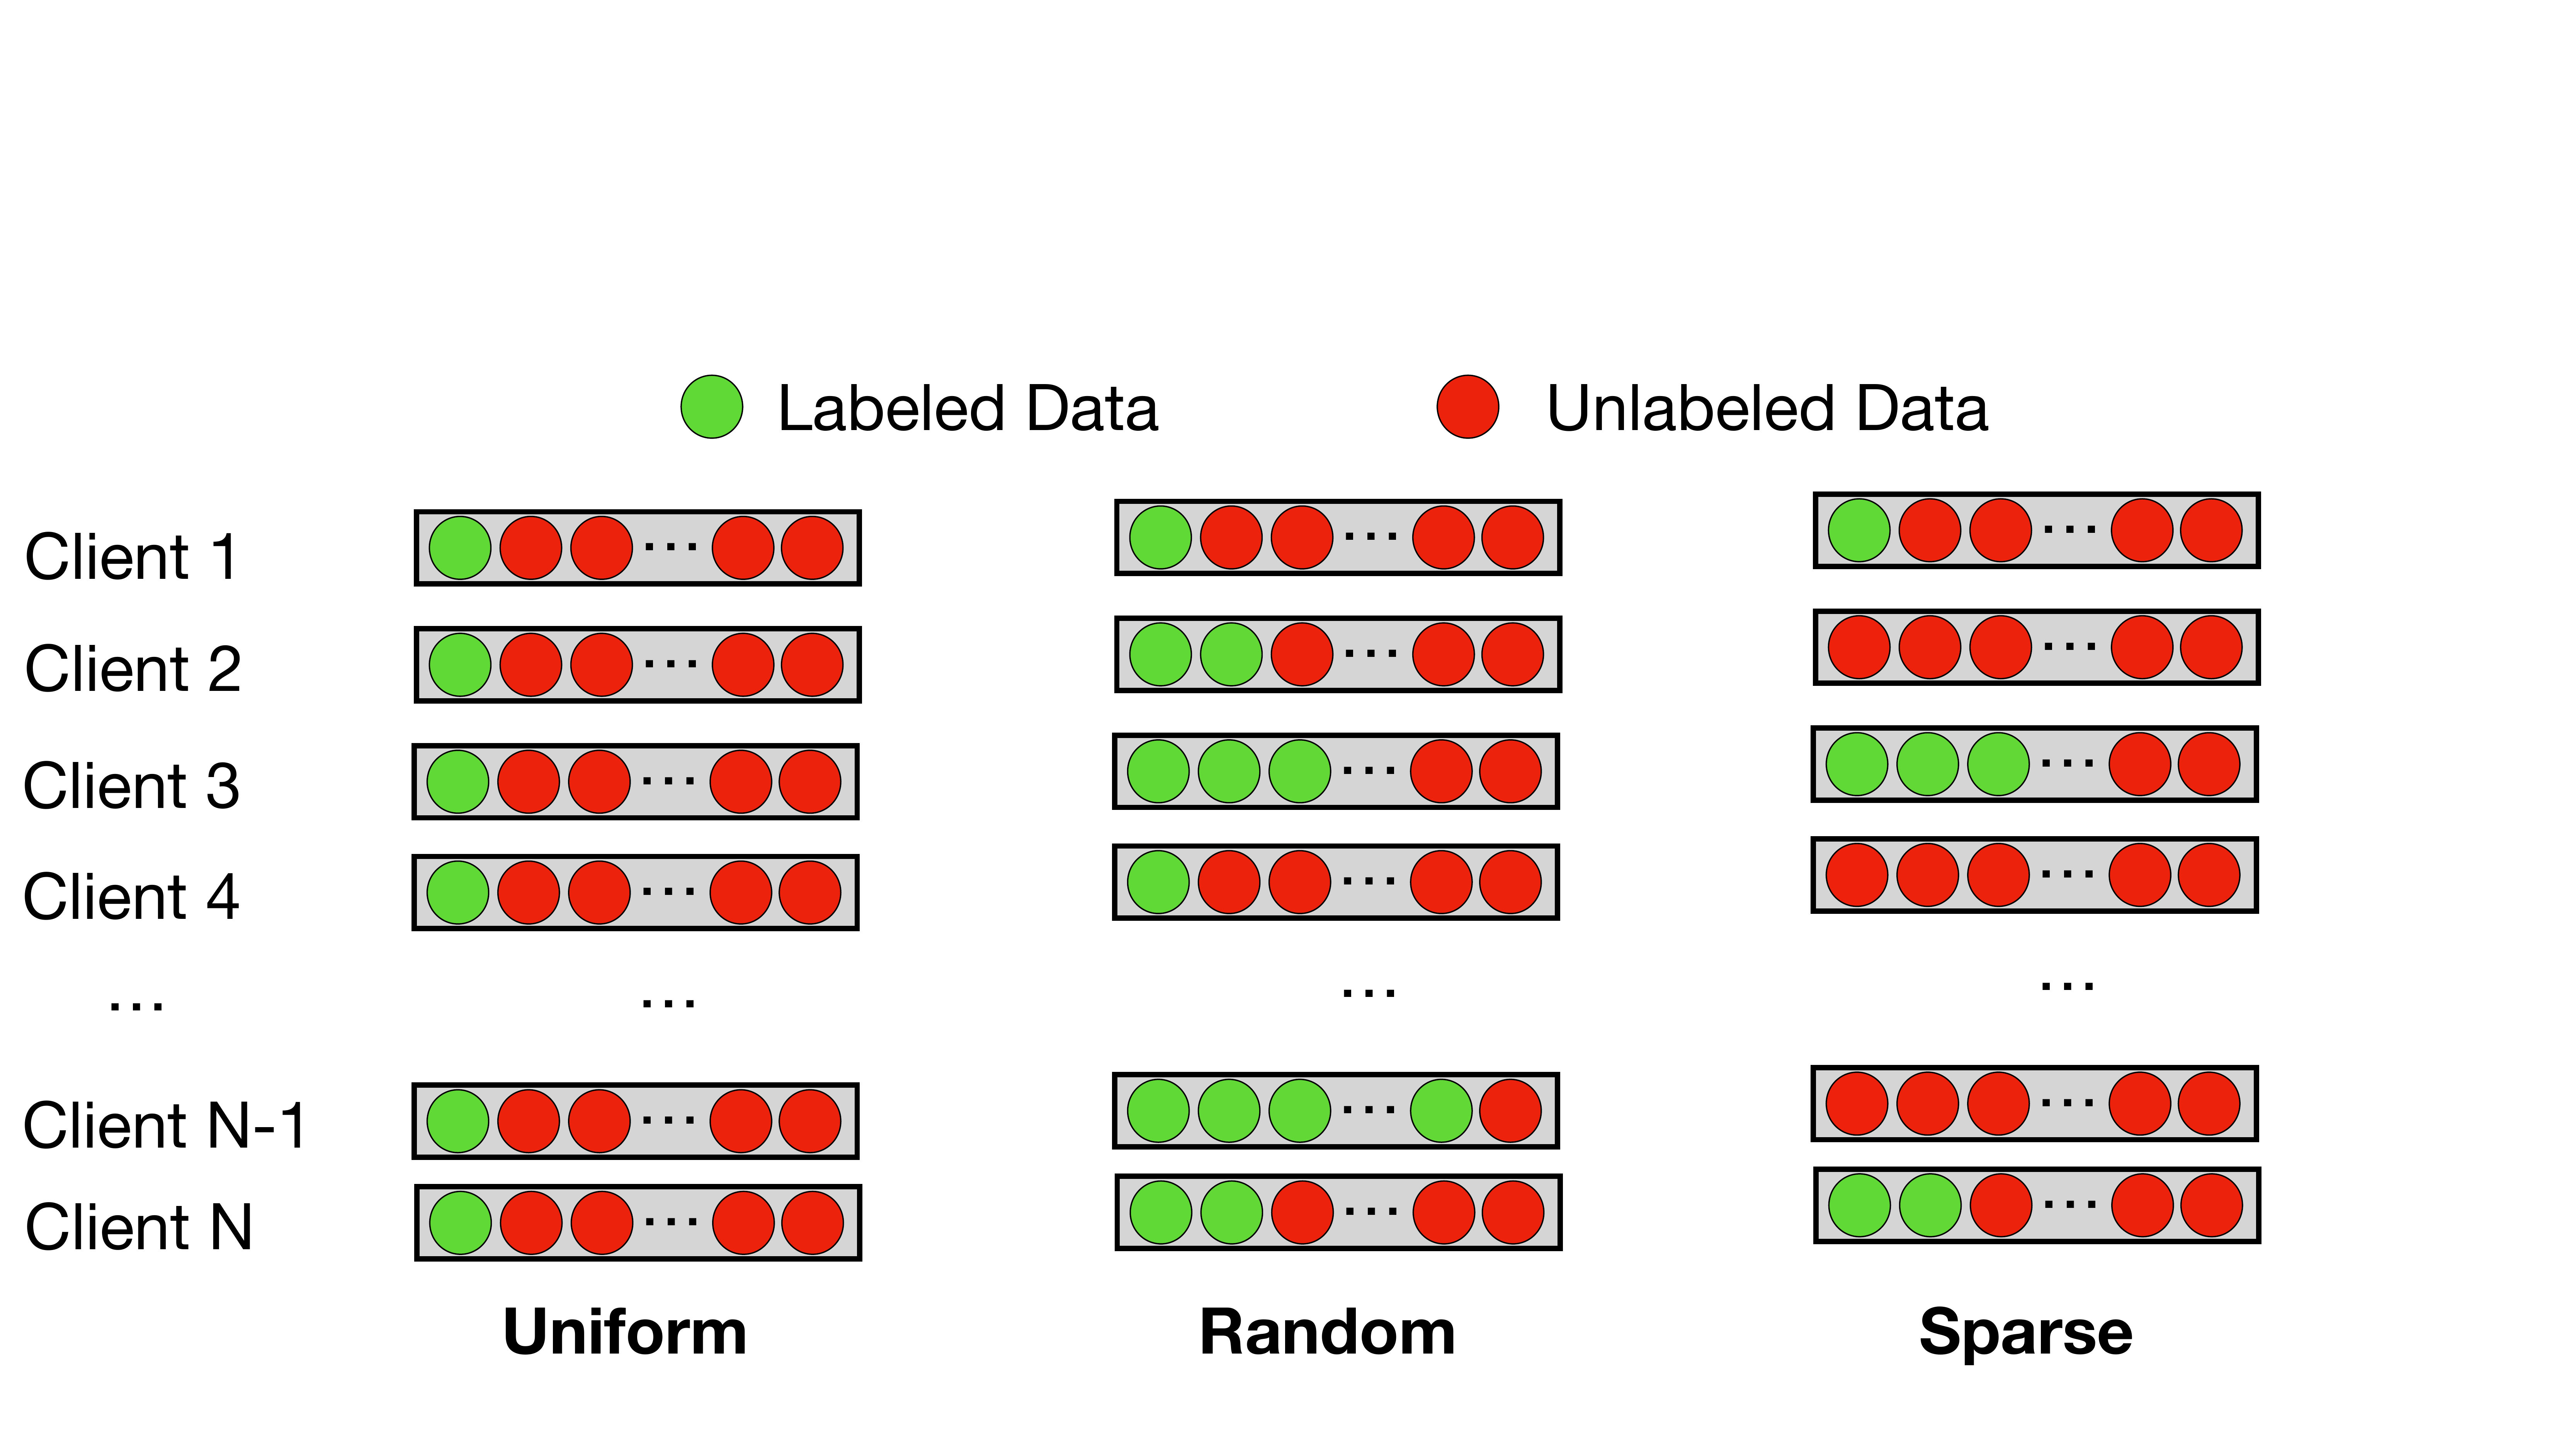}
	%  \vspace{-10pt}
	\caption{Different data distribution for FSL. \mwx{Should be replaced by a system design picture or system implementation comple workflow (including cloud pre-training, labeled data input and fine-tuning on mobile devices.).}} 
	% \vspace{-15pt}
	\label{fig:def-fsl-distribution}
\end{figure}

% \begin{figure}[t]
% 	\centering
% 	 \includegraphics[width=0.27\textwidth]{figs/design-adapter-arch.pdf}
% 	 \vspace{-5pt}
% 	\caption{The structure of adapters used.} 
% 	\vspace{-10pt}
% 	\label{fig:design-adapter-arch}
% \end{figure}

\begin{figure*}[t]
	\centering
        \includegraphics[width=0.6\textwidth]{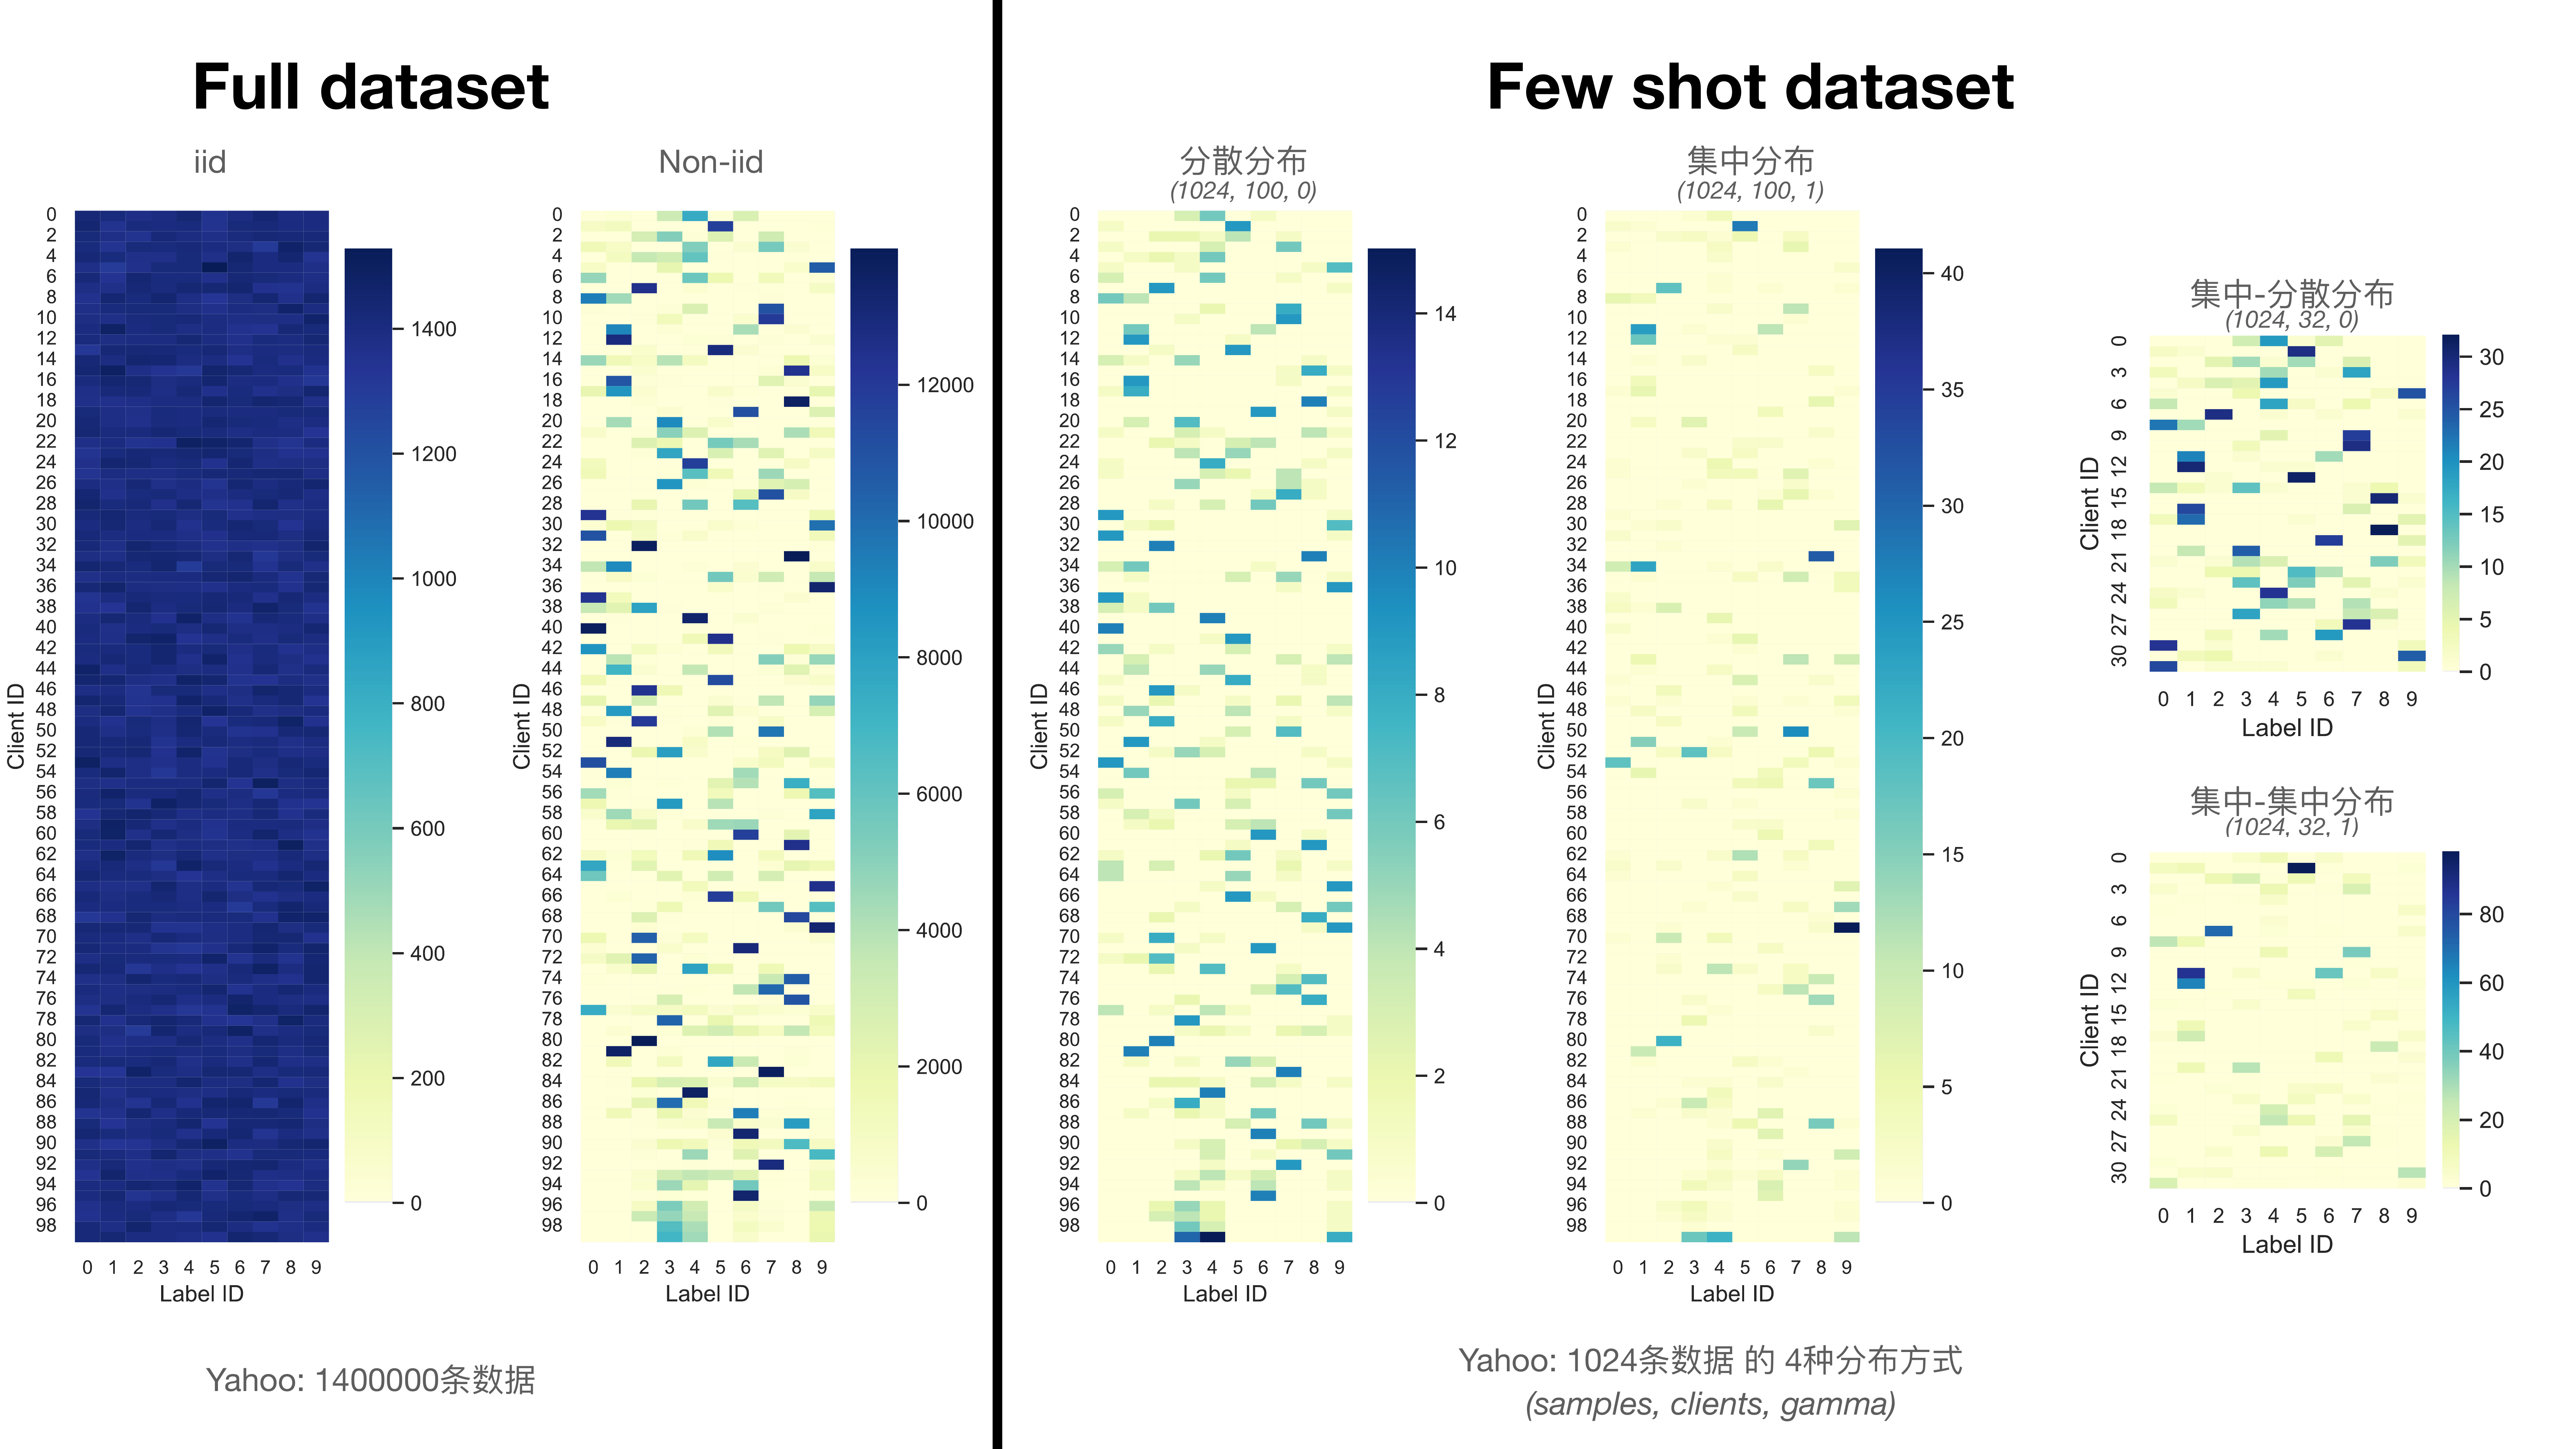}

	%  \vspace{-10pt}
	\caption{We define a new triple tuple (samples, clients, sparsity): noted as ($n$, $\xi$, $\gamma$) to represent the true few show learning (labeled) data distribution. \mwx{N-ways K-shots: way means number of labels, shot means data quantity for each label.}} 
	% \vspace{-15pt}
	\label{fig:def-distribution}
\end{figure*}
We follow the popular FedNLP framework~\cite{lin-etal-2022-fednlp} to use $\alpha$ to define \textbf{Non-IID Label Distributions.}
`12Here we present how we synthesize the data partitions such that clients the share same (or very similar) number of examples, but have different label distributions from each other.
We assume that on every client training, examples are drawn independently with labels following a categorical distribution over L classes parameterized by a vector q (qi $\geq$ 0, i $\in$  [1, L] and $‖q‖$ = 1). 
To synthesize a population of non-identical clients, we draw q $\sim$  DirL($\alpha$p) from a Dirichlet distribution, where p characterizes a prior class distribution over L classes, and $\alpha$ > 0 is a concentration parameter controlling the identicalness among clients. 
For each client $C_{j}$, we draw a $q_{j}$ as its label distribution and then sample examples without replacement from the global dataset according to $q_{j}$. 
With $\alpha$ $\rightarrow$ $\infty$ , all clients have identical distributions to the prior (i.e., uniform distribution); 
with $\alpha$ $\rightarrow$ 0, on the other extreme, each client holds examples from only one class chosen at random. 
As shown in Figure~\ref{fig:def-distribution}, we show a series heatmaps for visualizing the distribution differences between each client.
Figure~\ref{fig:def-gamma} shows an example of the concrete label distributions for all clients with different $\alpha$. 
We can see that when $\alpha$ is smaller, the overall label distribution shift becomes larger.

\subsubsection{Non-IID. Quantity Distribution}
\begin{figure}[t]
	\centering
	 \includegraphics[width=0.45\textwidth]{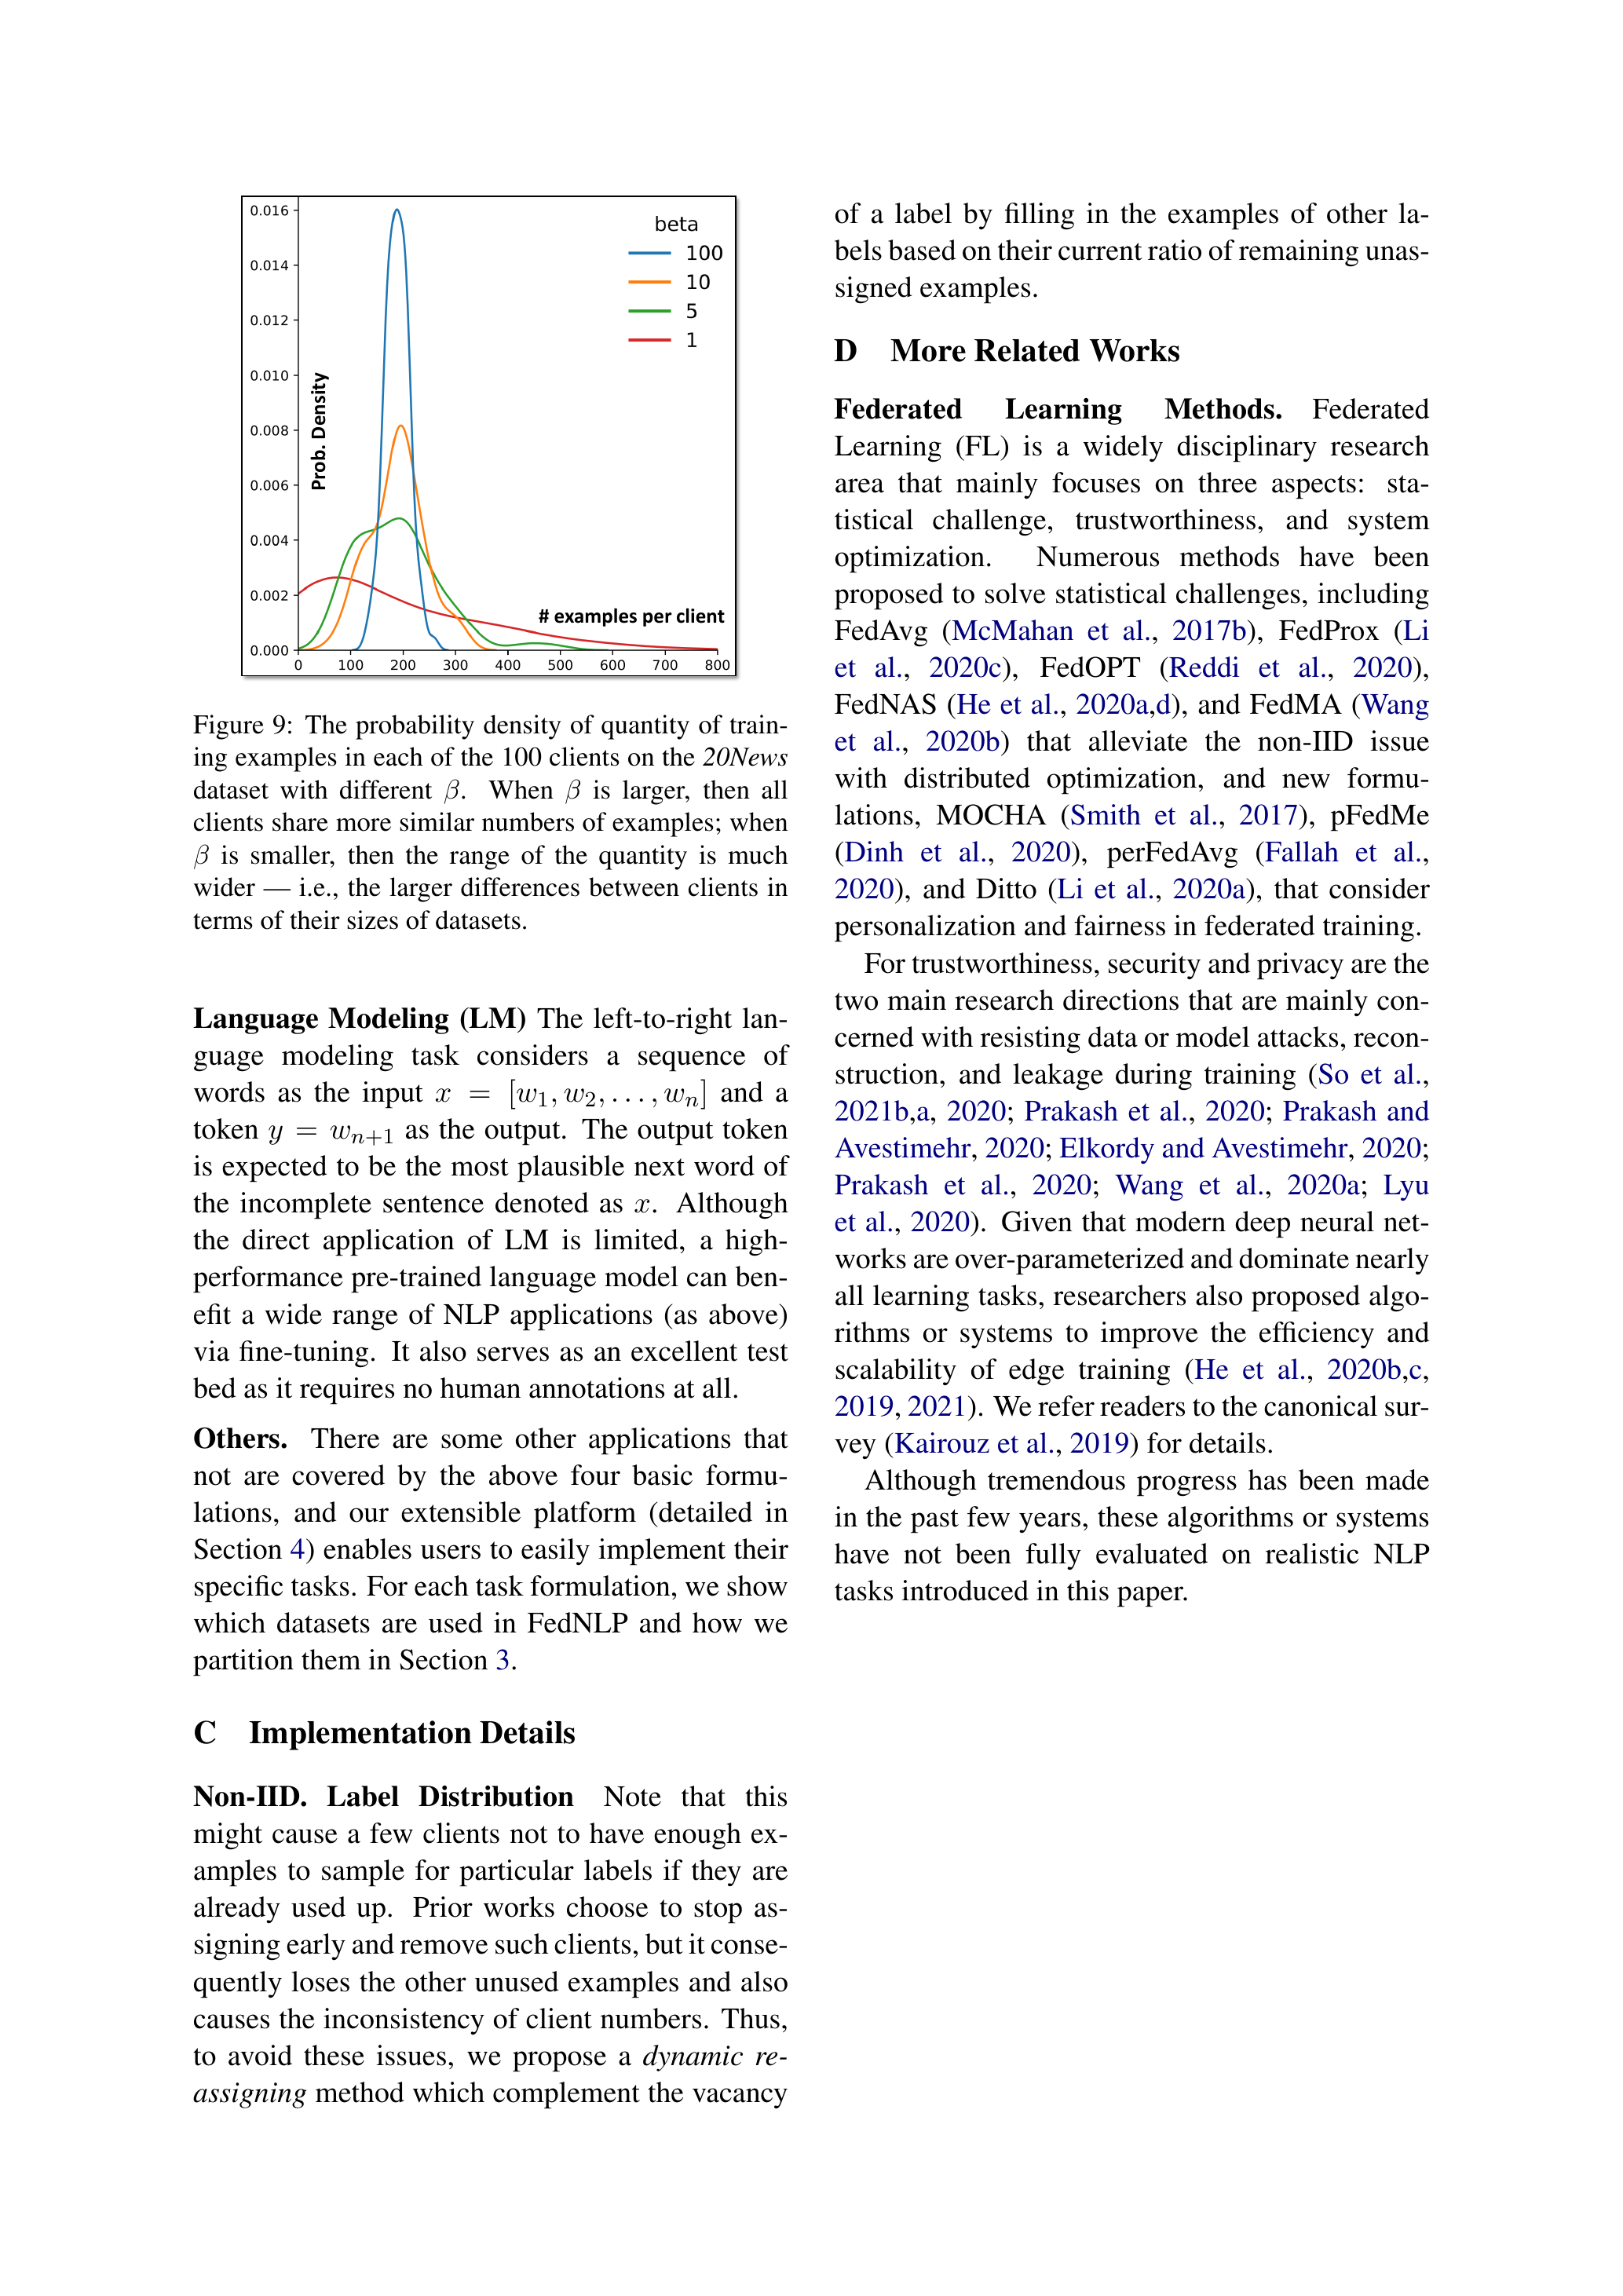}
	%  \vspace{-10pt}
	\caption{The probability density of quantity of training examples in each of the 100 clients on the 20News dataset with different $\beta$. When $\beta$ is larger, then all clients share more similar numbers of examples; when $\beta$ is smaller, then the range of the quantity is much wider — i.e., the larger differences between clients in terms of their sizes of datasets.} 
	% \vspace{-15pt}
	\label{fig:def-fednlp-beta}
\end{figure}
It is also common that different clients have very different data quantities while sharing similar label distribution. 
We thus also provide a quantity-level Dirichlet allocation $z$ $\sim$ DirN ($\beta$) where N is the number of clients. 
Then, we can allocate examples in a global dataset to all clients according to the distribution $z$ — i.e., |$D_{i}$| = $z_{i}$|$D_{G}$|. If we would like to model both quantity and label distribution shift, it is also easy to combine both factors. Note that one could assume it is a uniform distribution z $\sim$ U (N ), (or $\beta \rightarrow \infty$ ) if we expect all clients to share similar number of examples. A concrete example is shown in Figure~\ref{fig:def-fednlp-beta} (Appendix).
