# Supplementary material for: Towards Practical Few-shot Federated NLP
Source: arXiv:2212.00192 source file (2023-08-19)
Supplement: Supplementary file 2 [file sec-appendix-overall.tex]

\subsection{Overall Performance}\label{sec:appendix-overall}

\textbf{Gain and Gap}

This section will show two-fold comparison:

1. Show the gain of few shot fedpet (prompting fine-tuning) versus vanilla fedcls (i.e., head fine-tuning)~\cite{scao2021many}.

2. Show the gap from few shot fedpet versus full dataset fine-tuning.

End-to-end exps: convergence plots (line plot. X-axis: clock time; Y-axis: testing accuracy).

\textbf{Accuracy gain turns more obvious when labeled data is extremely few.} Accuracy gain means how much FedPrompt outperforms vanilla fine-tuning, shown in Figure~\ref{fig:eval-performance-gain}.

% \begin{figure}[t]
% 	\centering
%     \begin{minipage}[b]{0.23\textwidth}
%         \includegraphics[width=0.98\textwidth]{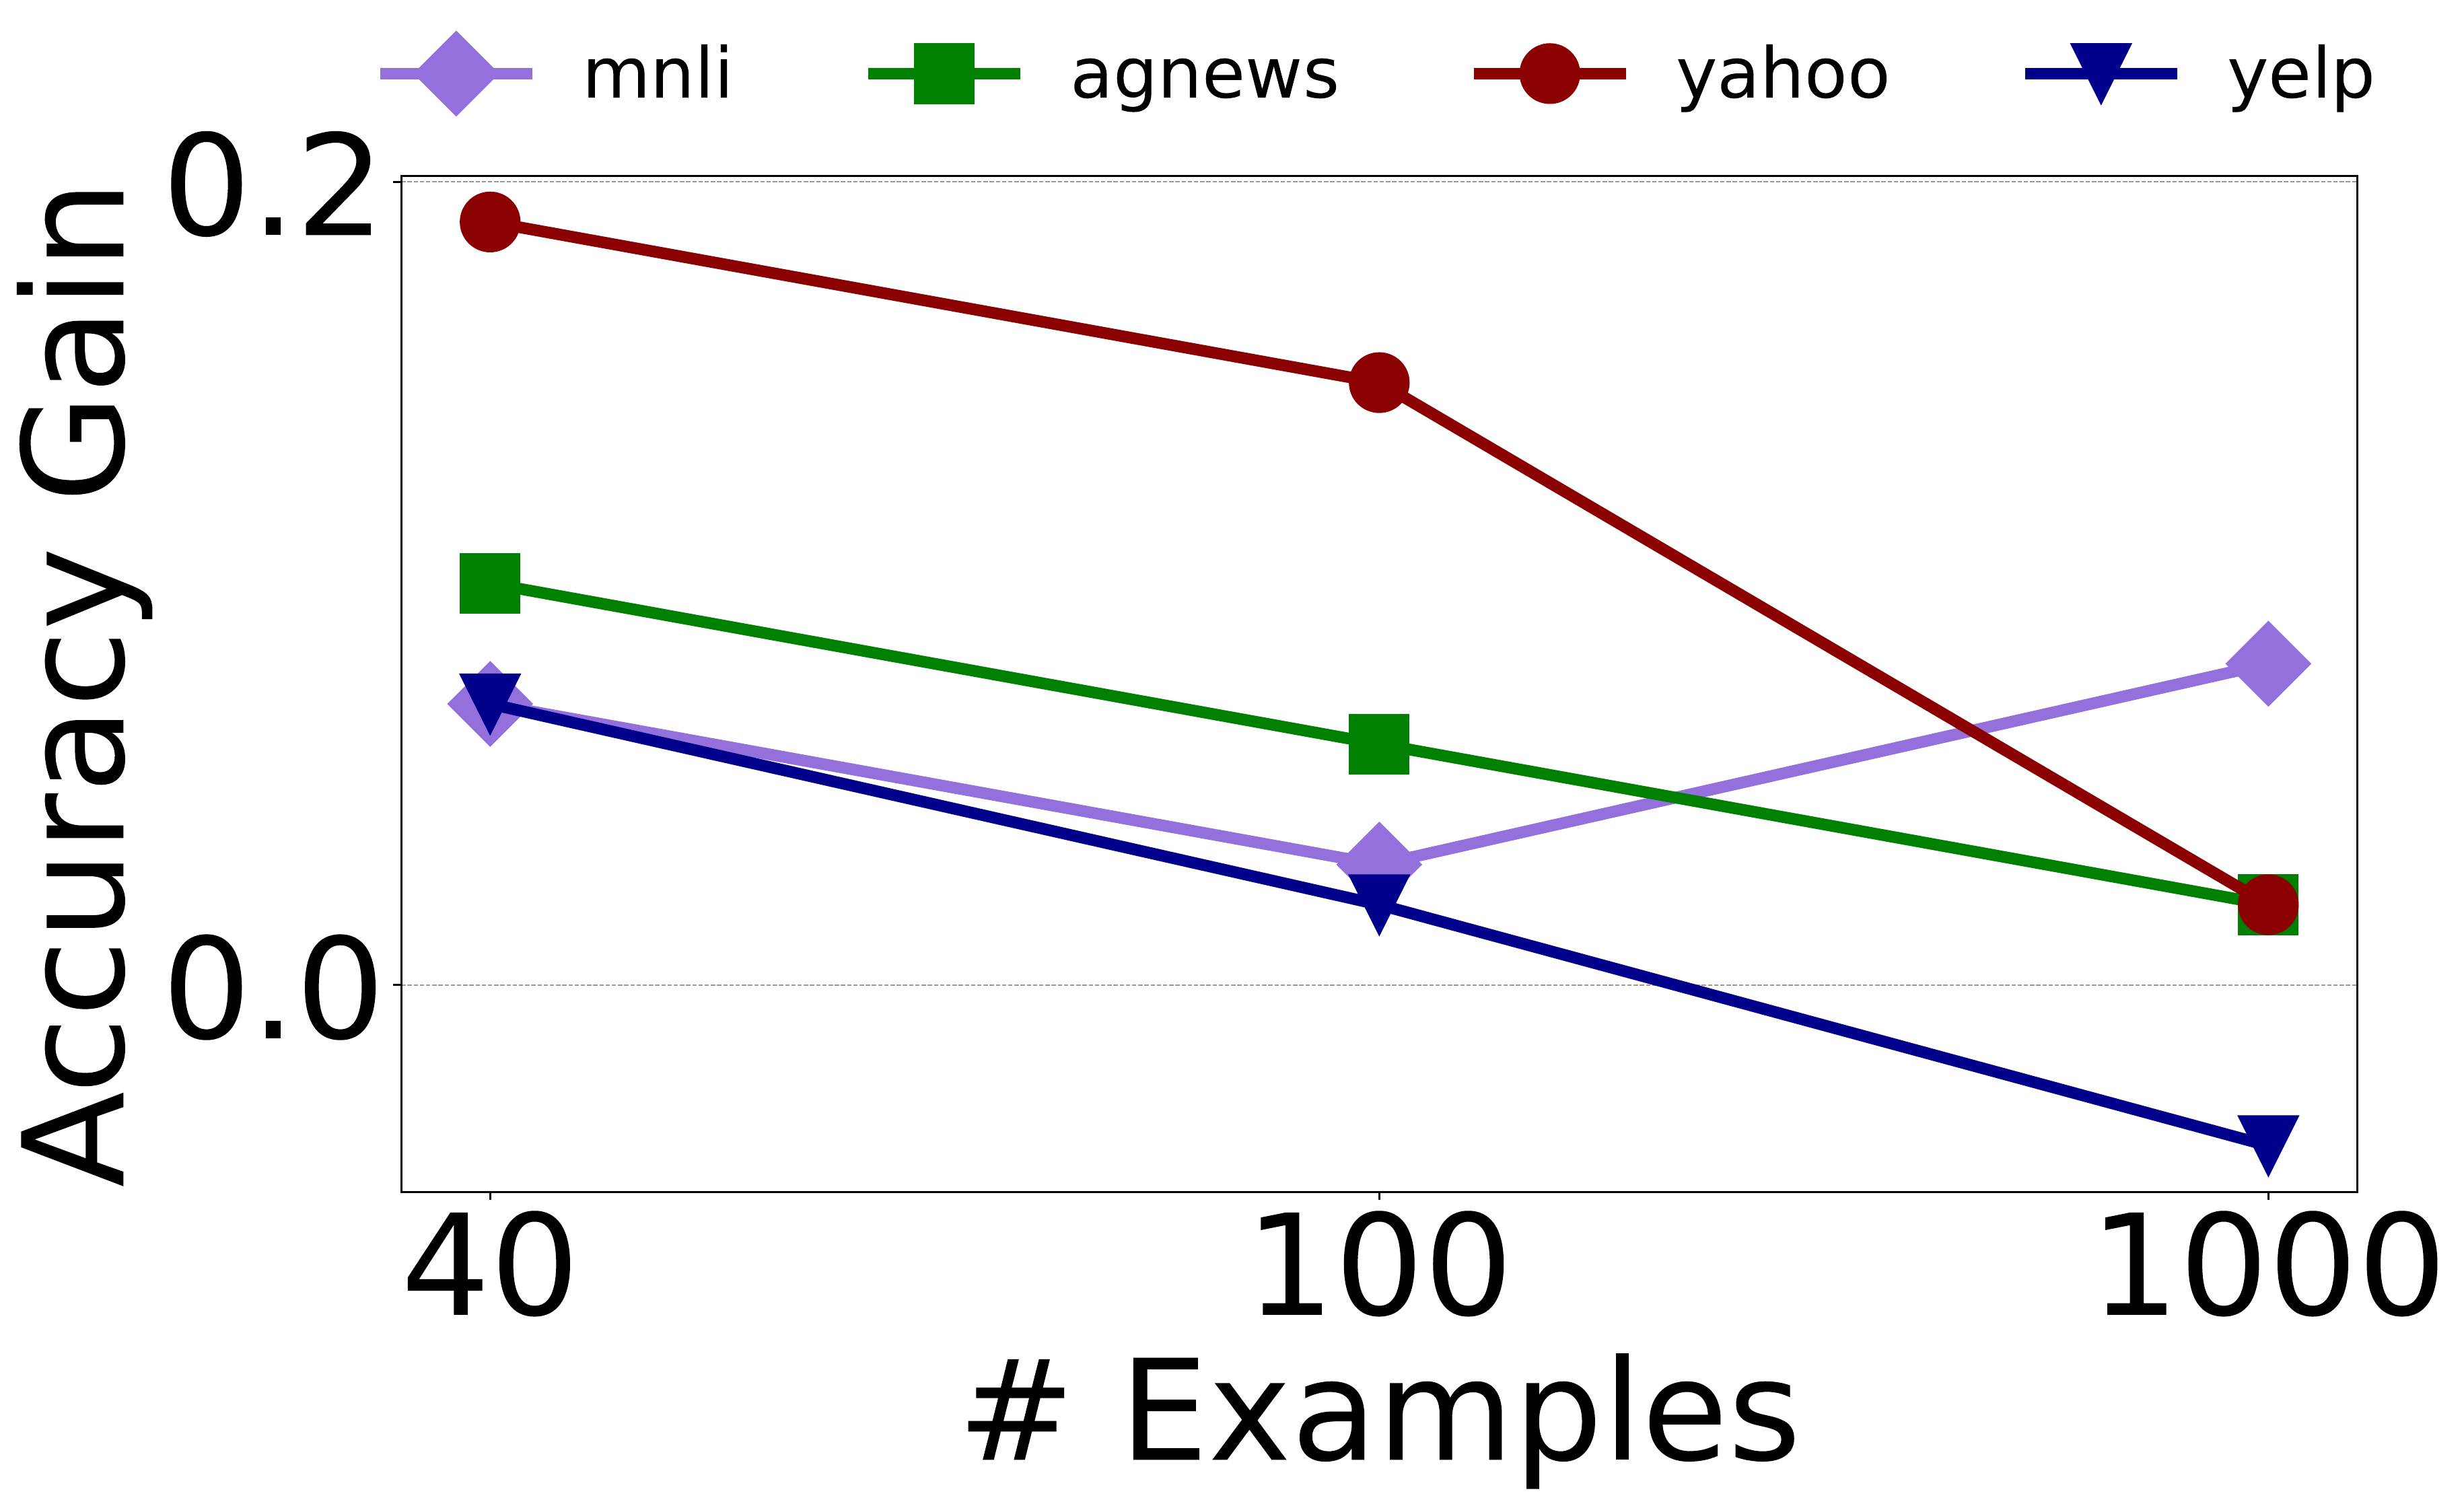}
%         \subcaption{AGNEWS}
%     \end{minipage}
%     ~
%     \begin{minipage}[b]{0.23\textwidth}
%         \includegraphics[width=0.98\textwidth]{figs/eval-performance-gain.pdf}
%         \subcaption{Dataset 2}
%     \end{minipage}
% 	%  \vspace{-10pt}
% 	\caption{Accuracy gain turns more obvious when labeled data is extremely few.} 
% 	% \vspace{-15pt}
% 	\label{fig:def-eval-performance-gain}
% \end{figure}

\begin{figure}[t]
	\centering
        \includegraphics[width=0.3\textwidth]{figs/eval-performance-gain.pdf}

	%  \vspace{-10pt}
	\caption{The conclusion of Figure~\ref{fig:eval-performance-overall}. Accuracy gain turns more obvious when labeled data reaching the `balance point'. Y-axis=Pet-CLS} 
	% \vspace{-15pt}
	\label{fig:eval-performance-gain}
\end{figure}

\textbf{There is a balance point for each dataset.}
\mwx{Simplify Figure~\ref{fig:eval-performance-overall} to one line. And parallel it with Figure~\ref{fig:eval-performance-gain}}
FedPrompt reaches its best gain when training setting is around the balance point.
Some balance point may be extremely few, e.g., AGNEWS.
While other datasets may need more labeled data to make the sufficient usage of the prompt to the pre-trained models.
Results are shown in Figure~\ref{fig:eval-performance-overall}.

\begin{figure*}[t]
	\centering
        \includegraphics[width=0.8\textwidth]{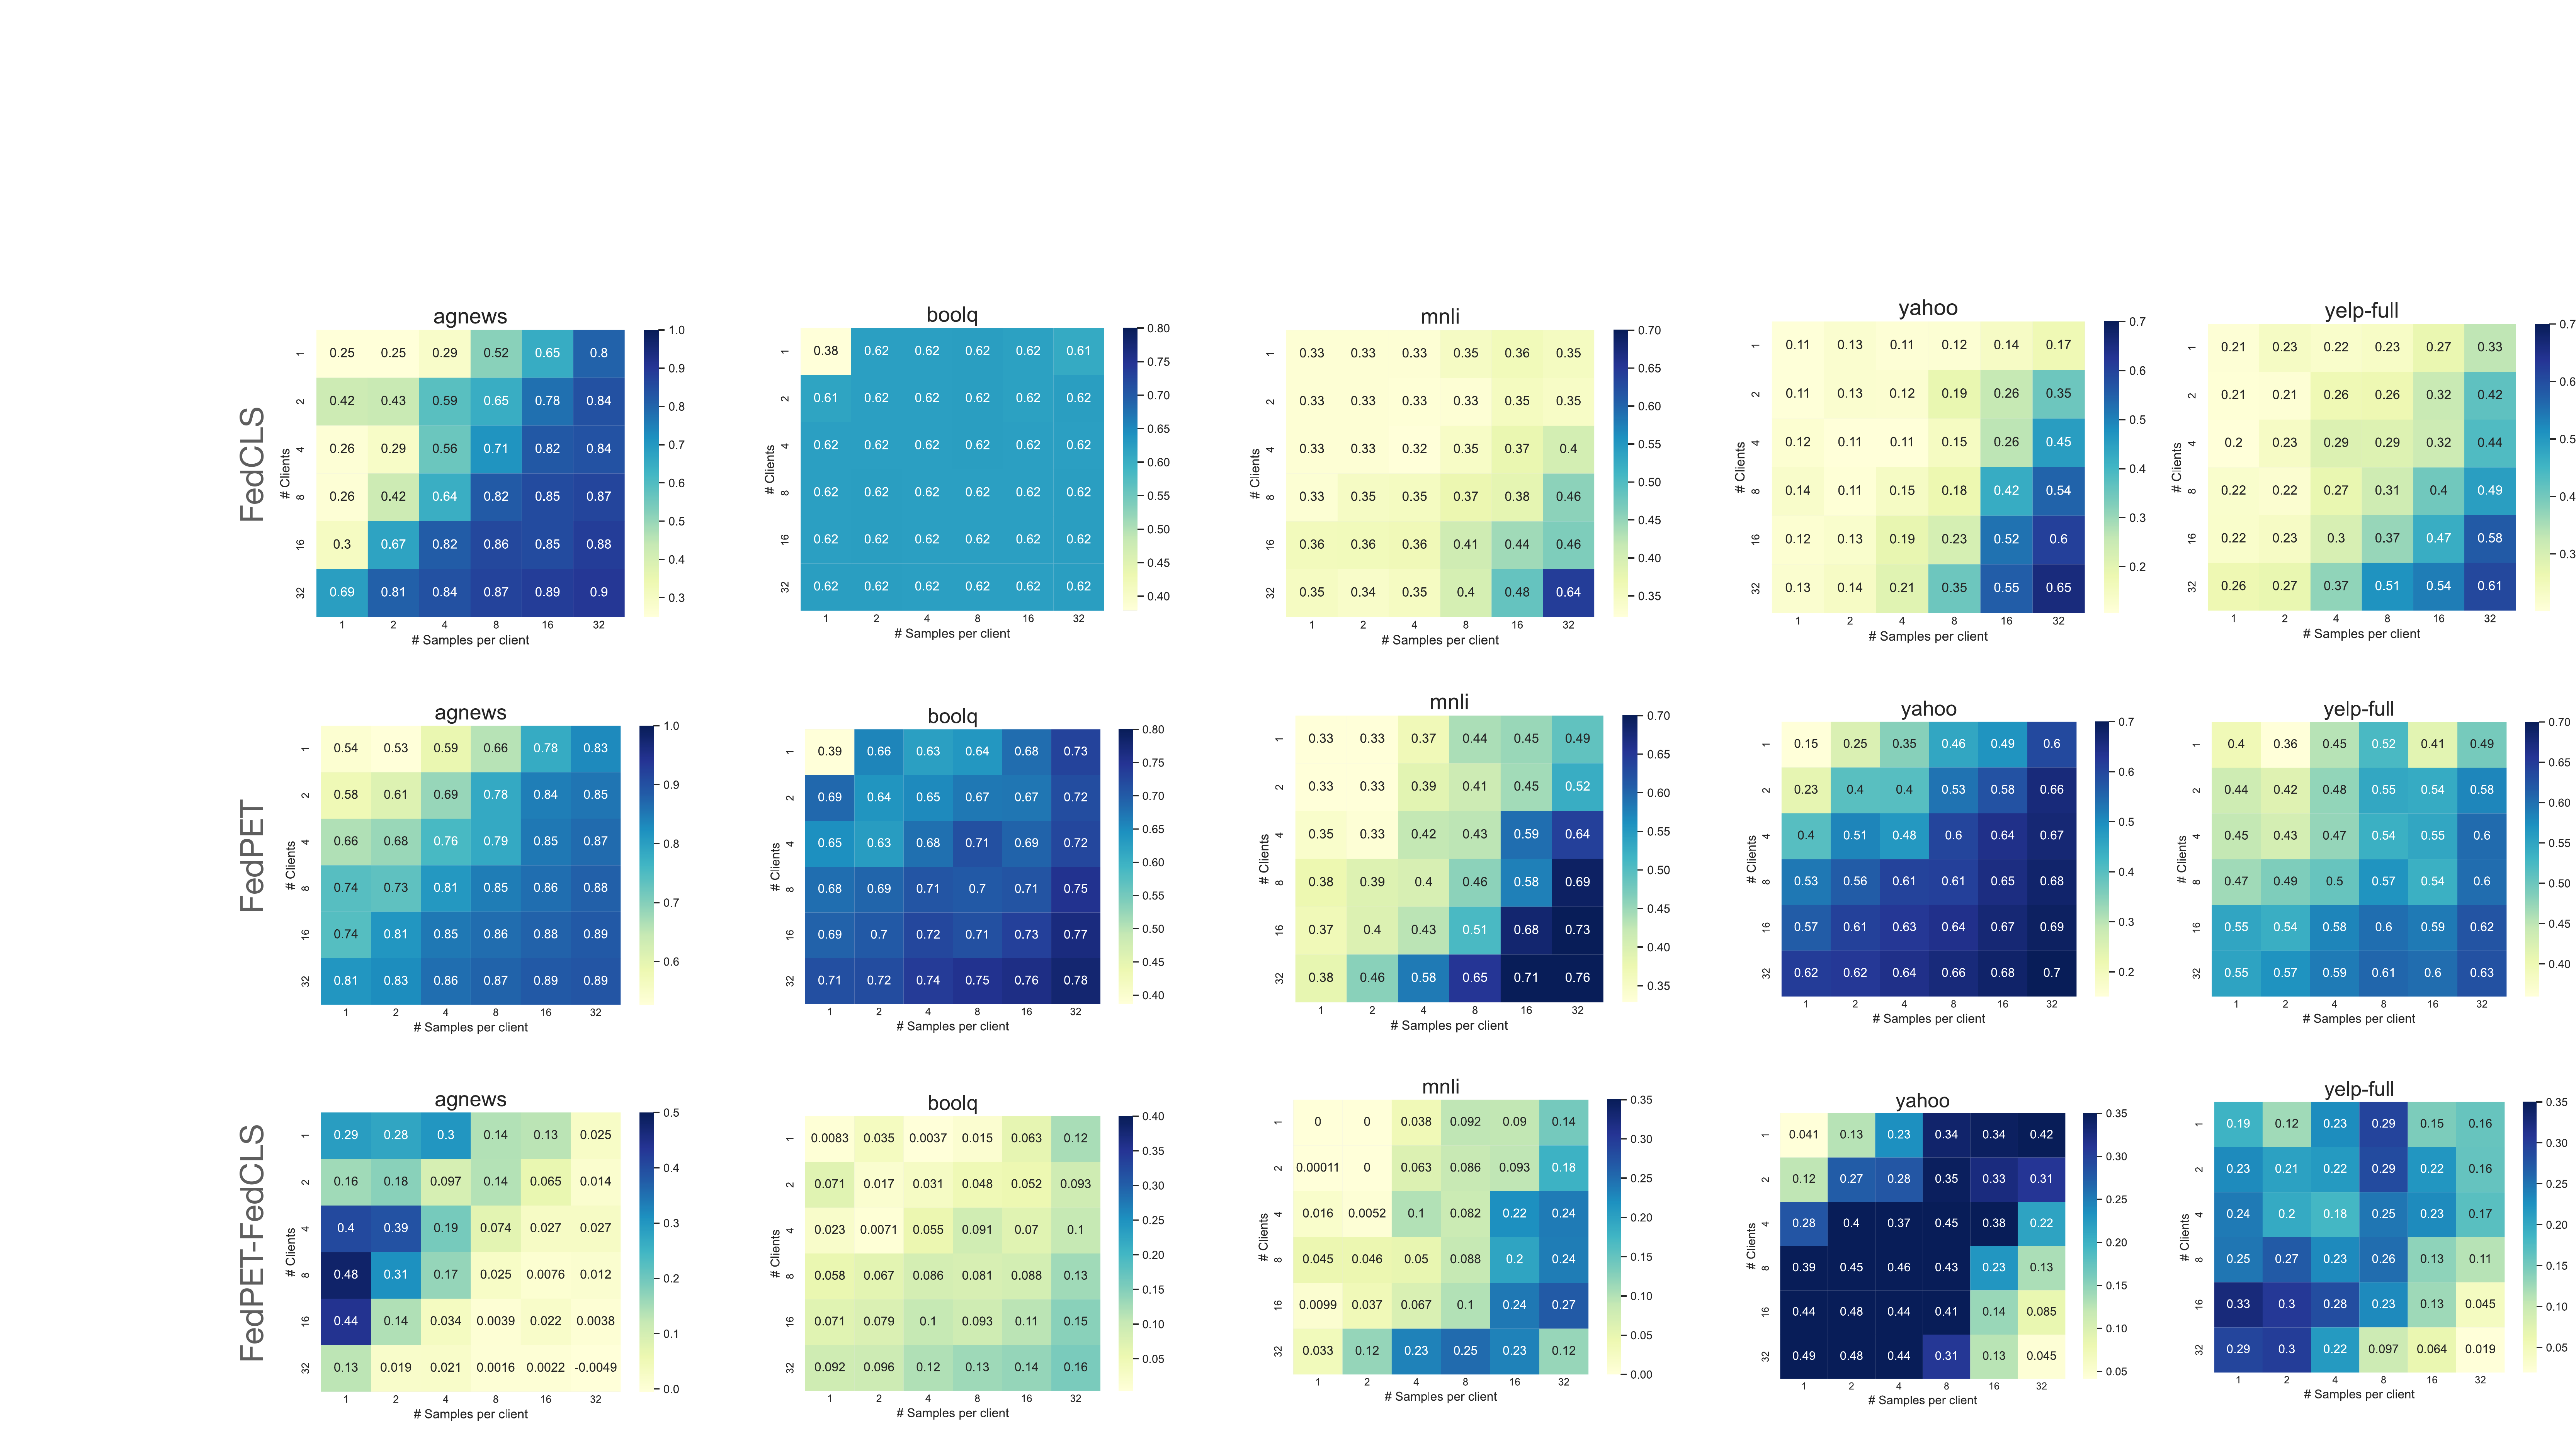}

	%  \vspace{-10pt}
	\caption{Balance point is different for various datasets. \mwx{Can be moved to appendix.}} 
	% \vspace{-15pt}
	\label{fig:eval-performance-overall}
\end{figure*}
