# Supplementary material for: Towards Practical Few-shot Federated NLP
Source: arXiv:2212.00192 source file (2023-08-19)
Supplement: Supplementary file 3 [file sec-appendix-sparsity.tex]

\subsection{Impact of Sparsity}\label{sec:appendix-sparsity}
Show all the datasets.

\begin{figure*}[t]
    \centering
    \begin{minipage}[b]{1\textwidth}
        \begin{minipage}[b]{0.24\textwidth}
            \includegraphics[width=0.95\textwidth]{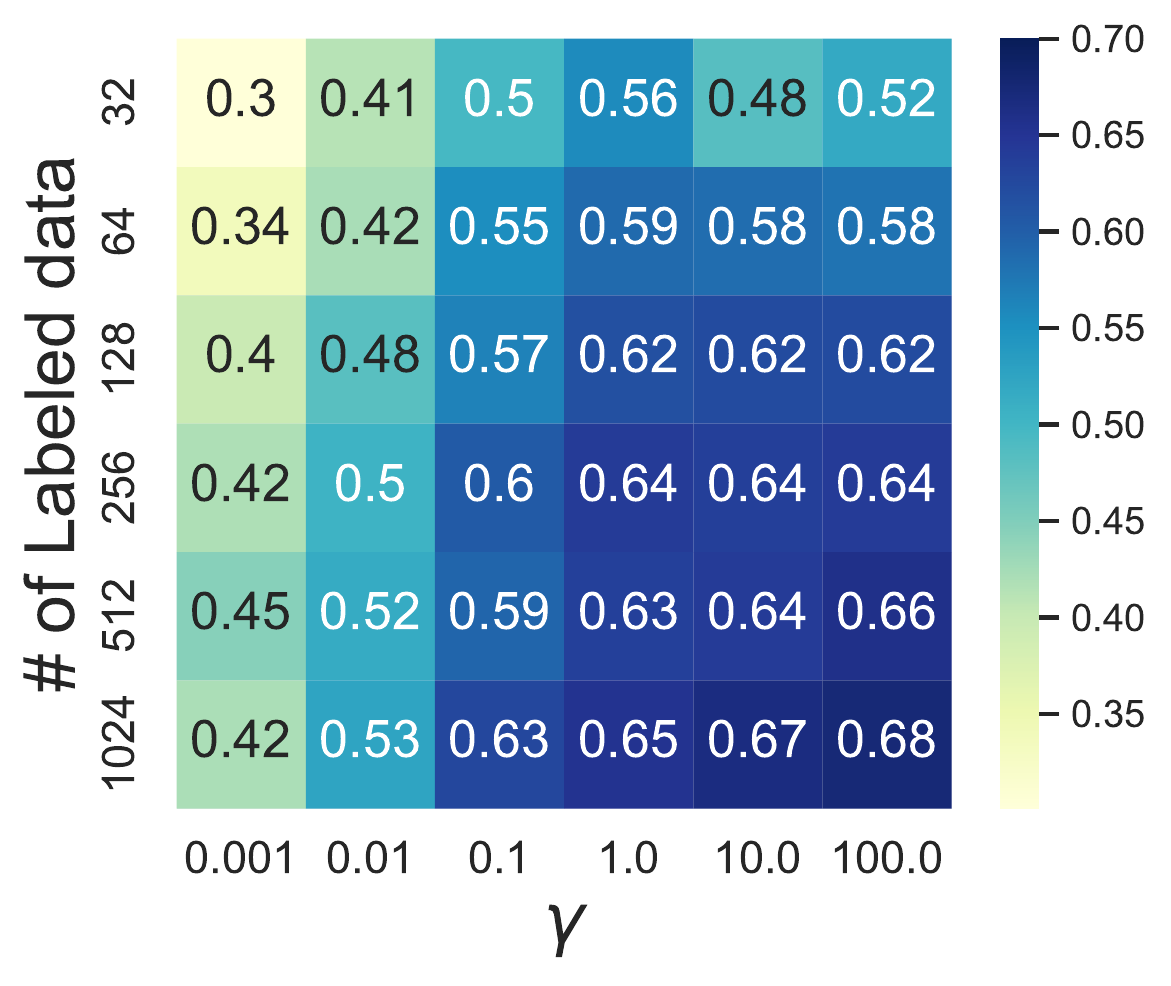}
            \subcaption{\texttt{YAHOO} (non-iid)}
        \end{minipage}
        ~
        \begin{minipage}[b]{0.24\textwidth}
            \includegraphics[width=0.95\textwidth]{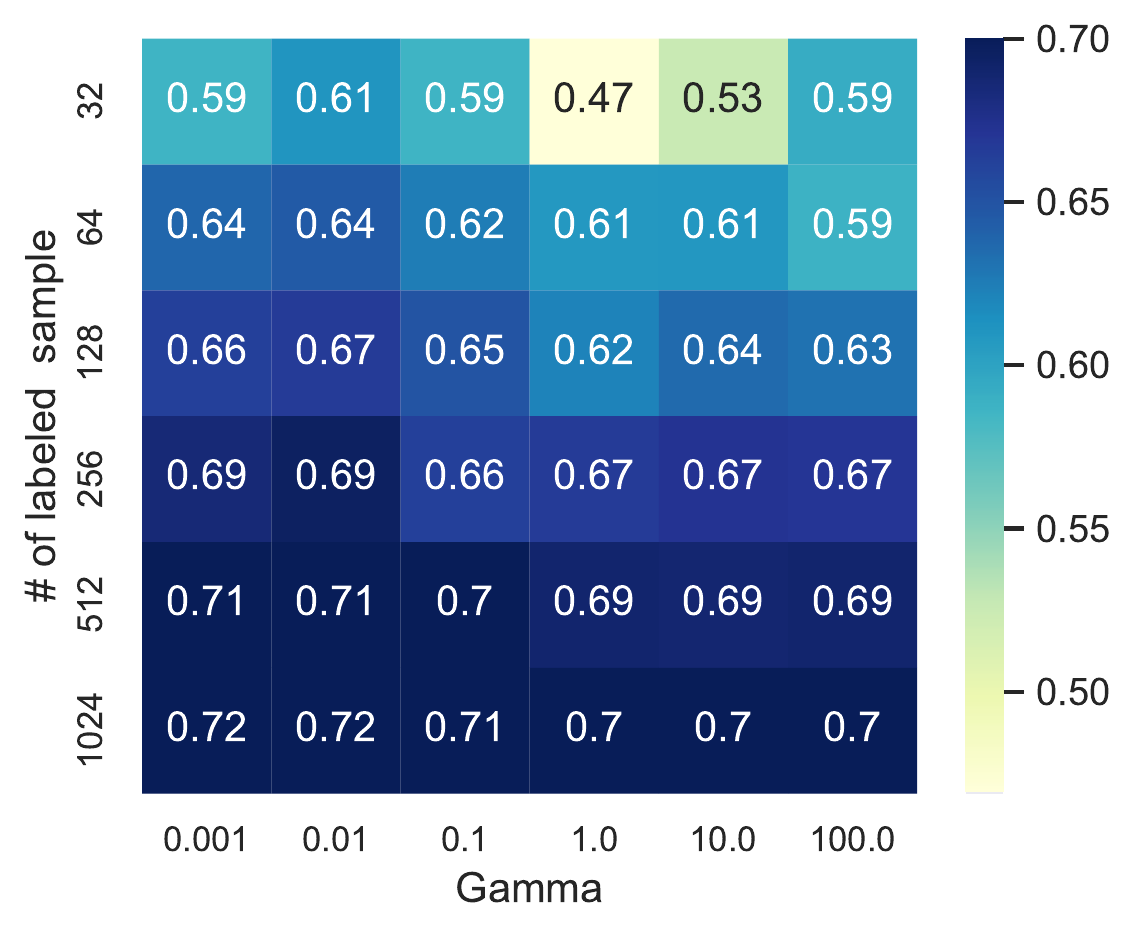}
            \subcaption{\texttt{YAHOO} (iid)}
        \end{minipage}
        ~
        \begin{minipage}[b]{0.24\textwidth}
            \includegraphics[width=0.95\textwidth]{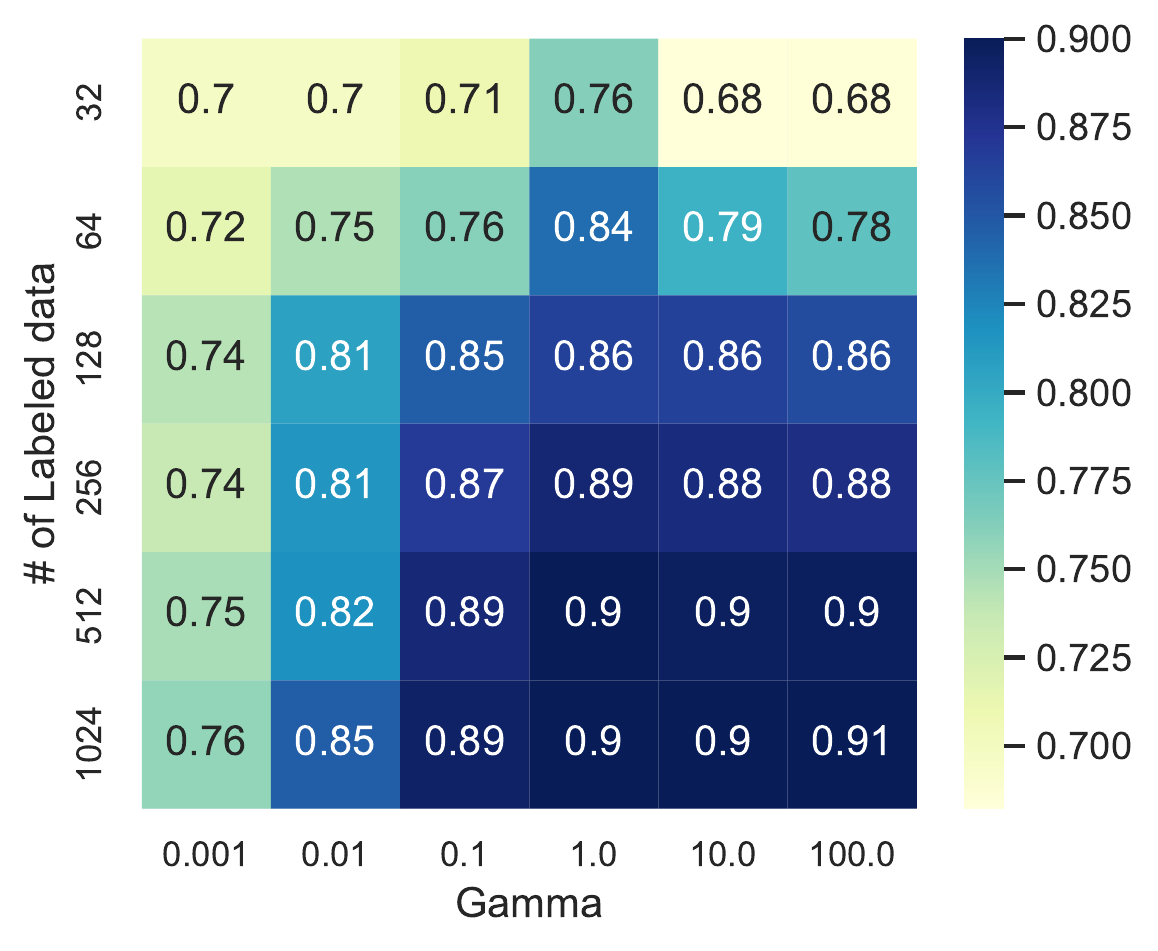}
            \subcaption{\texttt{AGNEWS} (non-iid)}
        \end{minipage}
        ~
        \begin{minipage}[b]{0.24\textwidth}
            \includegraphics[width=0.95\textwidth]{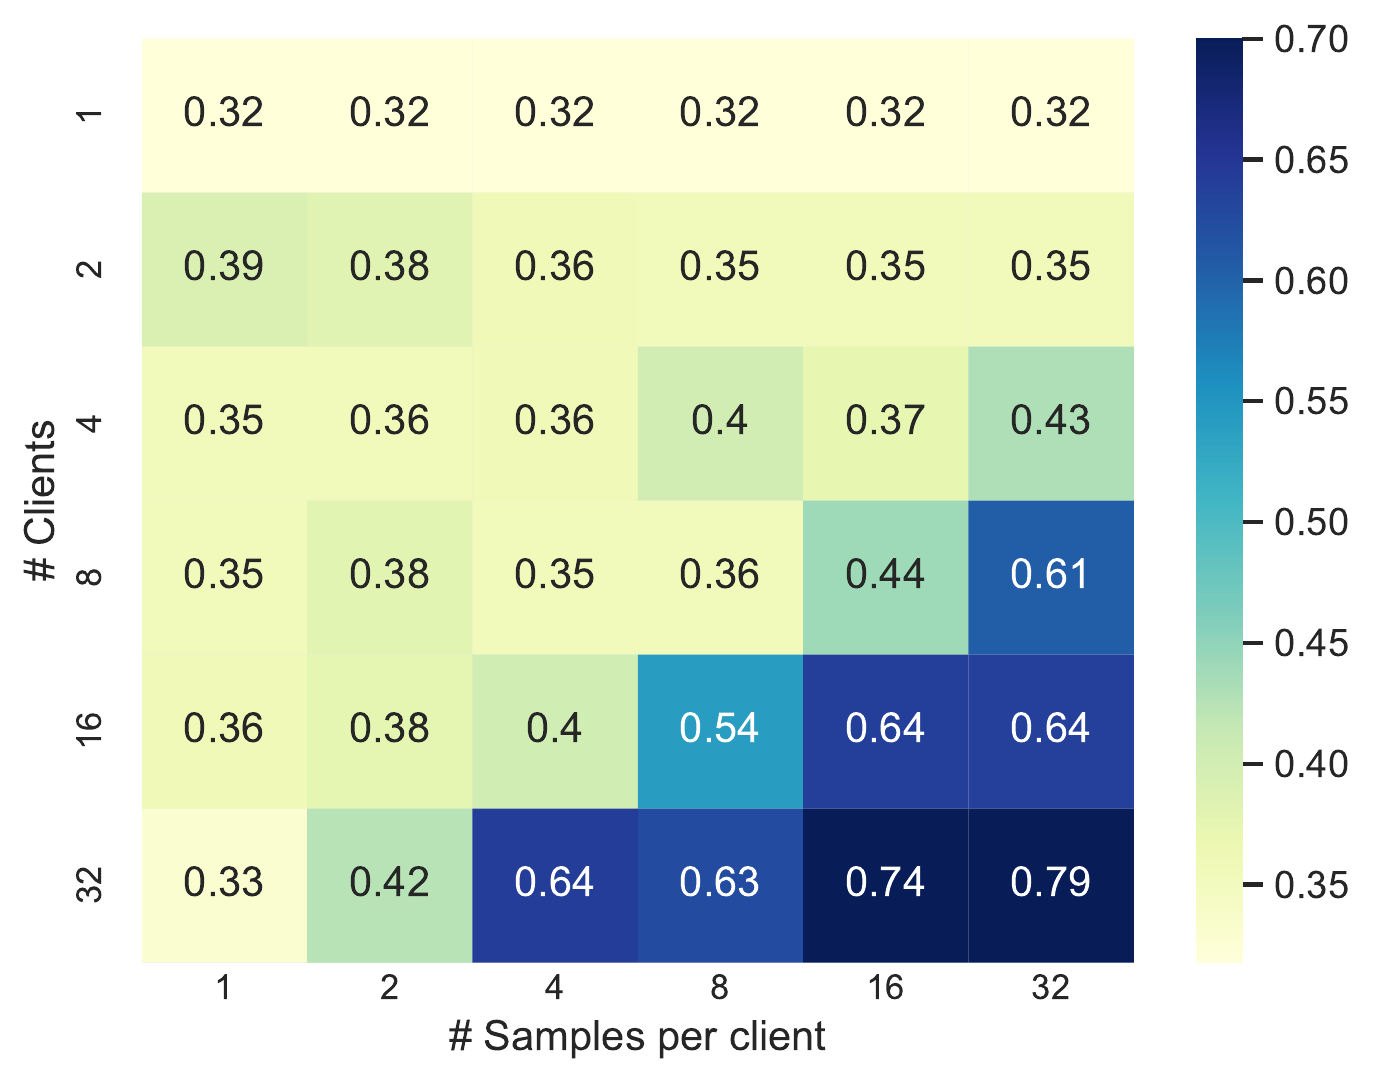}
            \subcaption{\texttt{MNLI} (non-iid)}
        \end{minipage}
    \end{minipage}
    
    \caption{(a). Scattered is better under non-iid distribution; (b). More data brings benefit; (c). new dataset; (d) impact of clients. \mwx{maybe just show fewer gamma case. It would be looking better.}}    
    \label{fig:eval-sparsity}
    
\end{figure*}

Result 1 is shown in Figure~\ref{fig:eval-sparsity}.

The combination of $clients$ and $\gamma$ controls the sparsity of labeled data.
We first fix the $clients$ being 32, and show performance with $\gamma$ growing up, i.e., labeled data is distributed more and more scattered.
As show in Figure~\ref{fig:eval-sparsity} (a,b,c), we get two interesting findings: 
1. when non-iid ($\alpha=1$), `Scattered is better';
2. when uniform ($\alpha \rightarrow \infty$), `More data is better regardless of labeled data distribution'.
Apart from that, we fix tha $\gamma$ be 1 (or 0), as show in Figure~\ref{fig:eval-sparsity} (d), we know that para. $clients$ do a great impact on the converge performance.
More labeled data distributed to more clients will bring significant improvement.
