# Supplementary material for: Towards Practical Few-shot Federated NLP
Source: arXiv:2212.00192 source file (2023-08-19)
Supplement: Supplementary file 4 [file sec-appendix.tex]

\section*{Appendix} \label{sec:appendix}

\subsection{Different Foundation Models}\label{sec:appendix-models}

\textbf{Performance under various foundation models:}
\mwx{Using 0.1\% data of full-set will enable BERT to perform on par on AGNEWS (0.6, 0.86), YAHOO(0.45, 0.66), YELP-F (0.27, 0.46), as well. While on MNLI, PET perform on par with CLS (0.48, 0.45). The Full-CLS are almost the same with Roberta-large.}

\input{fig-eval-model.tex}

\subsection{System Cost}

Performance of various models, shown in Figure~\ref{fig:eval-model}.

\mwx{Expected conclusion:} Large-scale foundation model is needed to take full advantage of prompt learning. 

\mwx{Show the runtime that arriving the 90\% of full-set accuracy.} Instead of the runtime line because the accuracy gap will confuse the reviewers.

Mobile device: Jetson TX2.

Latency and peak memory of different foundation models.

\mwx{Eval the impact of models.}
BERT: some datasets perform bad. But whether it can caused by the origin BERT feature instead of FedPET.
That is to say, those dataset perform bad on BERT even fine-tuned on full dataset.

MobileBERT, DistilBERT, etc.
\begin{itemize}
    \item Energy exps: per-device energy consumption at average till convergence (bar plot).
    
    \item Network exps: per-device network cost at average till convergence (bar plot).
    
    \item Memory exps.
\end{itemize}
