# Supplementary material for: Towards Practical Few-shot Federated NLP
Source: arXiv:2212.00192 source file (2023-08-19)
Supplement: Supplementary file 5 [file sec-appendix-models.tex]

\subsection{Different Foundation Models}\label{sec:appendix-models}

\textbf{Performance under various foundation models:}
\mwx{Using 0.1\% data of full-set will enable BERT to perform on par on AGNEWS (0.6, 0.86), YAHOO(0.45, 0.66), YELP-F (0.27, 0.46), as well. While on MNLI, PET perform on par with CLS (0.48, 0.45). The Full-CLS are almost the same with Roberta-large.}

\input{fig-eval-model.tex}
