# Supplementary material for: Towards Practical Few-shot Federated NLP
Source: arXiv:2212.00192 source file (2023-08-19)
Supplement: Supplementary file 6 [file sec-appendix-soft-label.tex]

\subsection{Softlabel}\label{sec:appendix-soft-label}

\textbf{Convergence accuracy:}

\textbf{Agnews (128 datapoints):} 

\textbf{Origin:} 90.3

\textbf{Augment:} 90.6

\textbf{Sparse Distribution ($\gamma$=0.001)} 71.3

\textbf{Augment: Sparse Distribution ($\gamma$=0.001)} 88.8

\textbf{Augment: Cold start ($\gamma$=0.001)} 25.0

% \textbf{Convergence accuracy:}

% \textbf{Yahoo (64 datapoints):} 

% \textbf{Origin:} 27.1

% \textbf{Augment:} 10.6

% \textbf{CorrectAugment:} 10.6

% \textbf{Sparse Distribution ($\gamma$=0.001)} 71.3

% \textbf{Augment: Sparse Distribution ($\gamma$=0.001)} 88.8

% \textbf{Augment: Cold start ($\gamma$=0.001)} 25.0

\mwx{Future work:}
1. Multi-pattern ensemble voting
2. Contrastive-Learning
